# Supplementary material for: Understanding Codebase like a Professional! Human-AI Collaboration for Code Comprehension
Source: arXiv:2504.04553 source file (2026-02-12)
Supplement: Supplementary file 1 [file appendix.tex]

\appendix

\section{Research Methods}
